# Supplementary material for: Label Noise in Adversarial Training: A Novel Perspective to Study Robust Overfitting
Source: arXiv:2110.03135 source file (2023-10-13)
Supplement: Supplementary file 1 [file 2.2-dependence.tex]

% \section{Data-dependent double descent in adversarial training}
% lucas
% \subsection{Data Matters for Double Descent in Adversarial Training}
% \label{sect:factor}

\subsection{Dependence of epoch-wise double descent in adversarial training}
\label{sect:double-descent-adversarial}
\todo{Remove first two, already discussed in the main paper}

\input{appendix/2-experiments/2.7-data-quality}

% \smallsection{Dependence of double descent on the data quality}

% \begin{figure*}[!ht]
%   \centering
%   \includegraphics[width=0.9\textwidth]{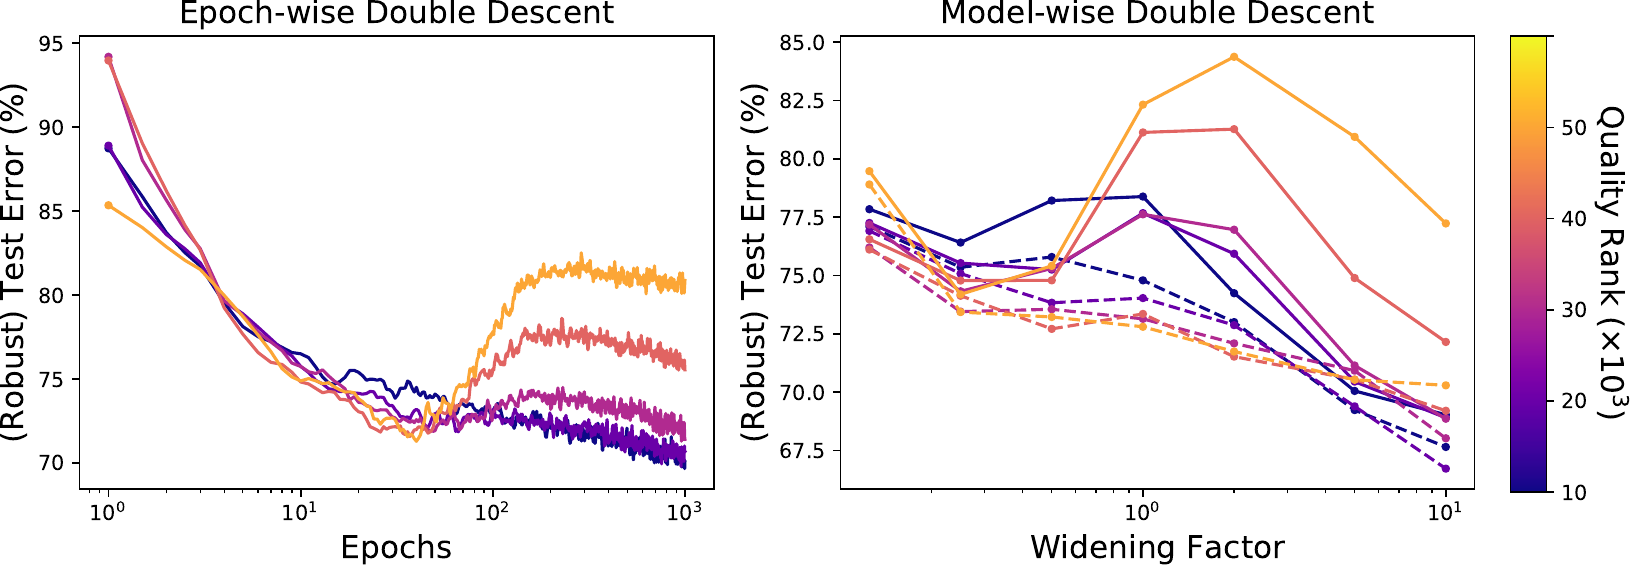}
%   \caption{Dependence of double descent on the data quality. As the quality of training data in adversarial training degrades, both the epoch-wise and model-wise double descent become more prominent. In the epoch-wise double descent figure, We smooth each curve by a window of 5 epochs to reduce the overlapping area. For the model-wise double descent the test error at the last checkpoint (solid line) and the test error at the best checkpoint (dashed line) are both shown. 
%   }
% \label{fig:dependence-data}
% \end{figure*}

% \chengyu{Need to run the experiments again}

% ===============================================
\smallsection{The number of attack iterations}
We have shown that the double descent in adversarial training strongly depends on the perturbation radius and the data quality. In this section we conduct experiments to show whether it also depends on the strength of the adversary. 
% A popular understanding of robust overfitting is the model overfits the adversarial perturbation as the inner maximization problem in adversarial training might not be sufficiently solved. However, in this section we modulate the strength of the adversary and show this is not the case.

In Figure~\ref{fig:dependence-iteration}, we fix the perturbation radius as $4/255$ where the double descent is relatively complete and vary the number of attack iterations of the PGD attack employed in the inner maximization. One may find that as long as the model capacity is reasonably large, the number of attack iterations will not significantly affect the double descent curve.
% , both for epoch-wise one and model-wise one. 
From the analysis of implicit label noise, this is easy to understand as more attack iterations will not reduce the probability corresponding to the true label much more---it is widely observed more iterations in PGD attack only marginally increase the attack successful rate. Consequently, the distribution mismatch between the true label distribution and the assigned label distribution that induces the implicit label noise will not expand significantly.

% \todo{Remove model-wise}
\begin{figure*}[!ht]
  \centering
  \includegraphics[width=0.45\textwidth]{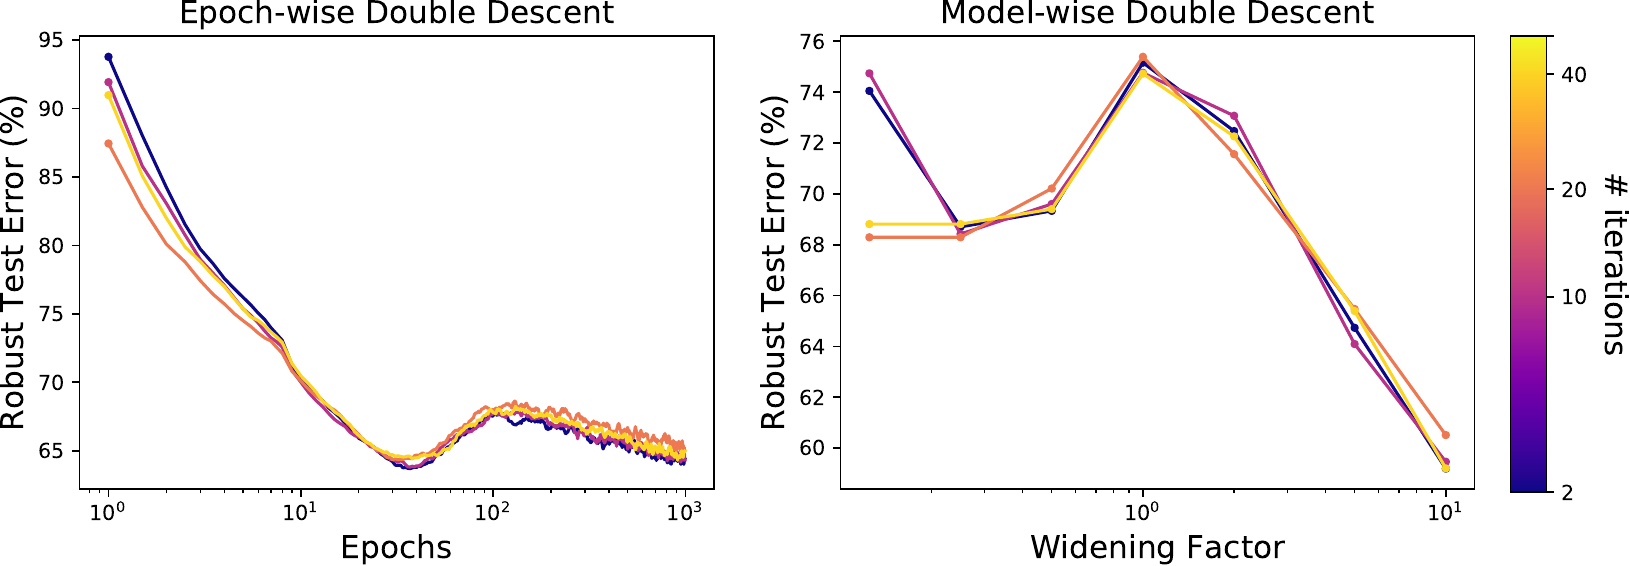}
  \caption{Dependence of epoch-wise double descent on the number of attack iterations. As more iterations are employed in the inner maximization, there is no significant change on epoch-wise double descent.
  }
\label{fig:dependence-iteration}
\end{figure*}

% \smallsection{Use AutoAttack for training}
% * AutoAttack is stronger than PGD-1000 (\cite{}).
% * Due to computation constraint, we adopt the regular training setting for this one.
% * An evidence showing that robust overfitting is not due to the model overfits weak perturbation (\cite{}?)
