# Supplementary material for: Label Noise in Adversarial Training: A Novel Perspective to Study Robust Overfitting
Source: arXiv:2110.03135 source file (2023-10-13)
Supplement: Supplementary file 2 [file 2.3-modelwise.tex]

\subsection{Model-wise double descent in adversarial training}
\label{sect:model-wise-double-descent}
\todo{Move model-wise of number of attacks in the above to here}

We have shown that the epoch-wise double descent, which is connected to the robust overfitting, is strongly dependent on the data. Here we show that the model-wise double descent, a parallel type of double descent, is dependent on the data in a similar manner. This is thus aligned with our theoretical analysis of the dependence of the implicit label noise.

In Figure~\ref{fig:dependence-model-wise-perturbation-quality}, we control the model capacity by modulating the widening factor of a Wide ResNet, and produce the model-wise double descent by picking the robust test accuracy at the last checkpoint. One can find the model-wise double descent becomes more significant as the perturbation radius increases. Interestingly, when the perturbation radius is smaller than $4/255$, the robust overfitting gap (the gap between the last error and the best error obtained throughout the training) will eventually close as the model capacity is sufficiently large. This is consistent with the phenomenon observed in the epoch-wise double descent that the last error will be as low as the best error when the perturbation radius is small. 
% since large model will be effectively over-parameterized at the very beginning of the training.
One can expect the same phenomenon happens for a typical perturbation radius such as $8/255$ with extremely large models. This suggests the robust overfitting might not be inevitable as claimed in previous works~\citep{Rice2020OverfittingIA}, but just because the current model in practice is still under-parameterized for adversarially robust learning. 

Similarly, the model-wise double descent also becomes more significant as the data quality degrades. When the data quality is high, the robust overfitting gap is also gradually closed as the model capacity increases. % Similar observation has been made in recent works~\citep{Dong2021DataPF}.
% These suggest that the robust overfitting is only transient in terms of both the training time and the model capacity.

\begin{figure*}[!ht]
  \centering
  \includegraphics[width=0.9\textwidth]{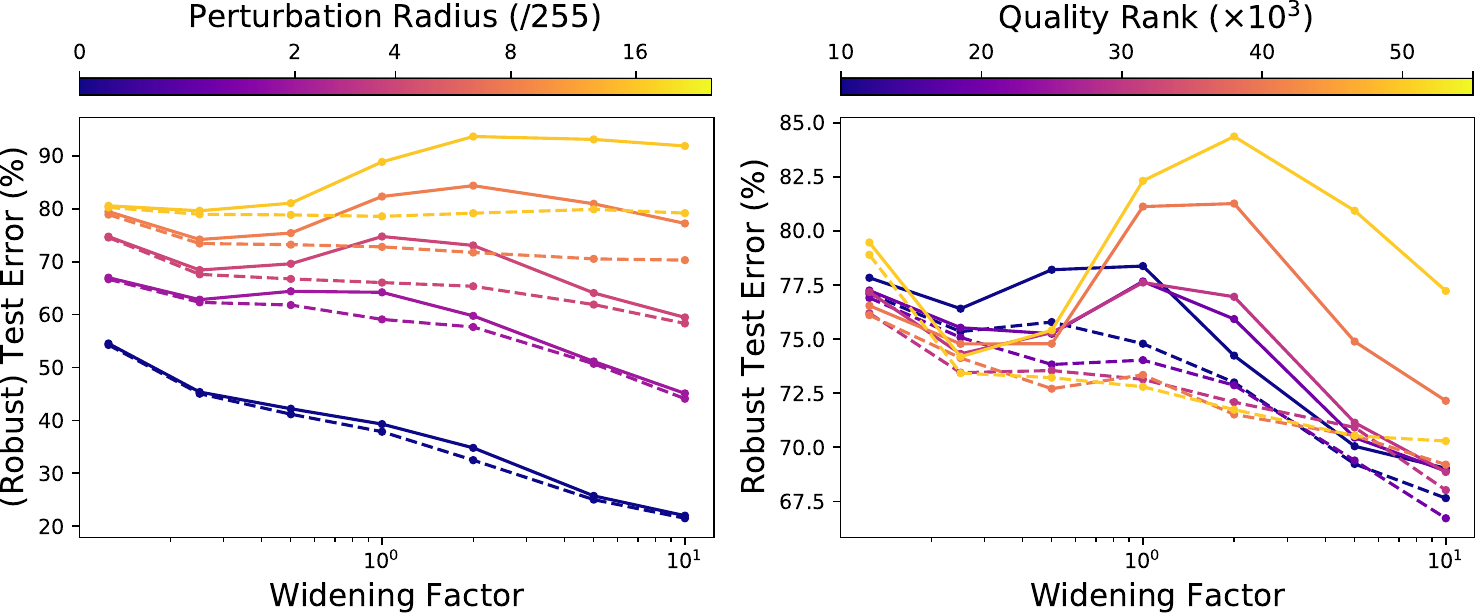}
  \caption{(Left) Dependence of model-wise double descent on the perturbation radius. 
  $\varepsilon = 0/255$ indicates the standard training where no double descent occurs. 
  (Right) Dependence of model-wise double descent on the data quality. The solid and dashed curves indicate the error at the best and last checkpoints, respectively.
  }
\label{fig:dependence-model-wise-perturbation-quality}
\end{figure*}
