# Supplementary material for: Label Noise in Adversarial Training: A Novel Perspective to Study Robust Overfitting
Source: arXiv:2110.03135 source file (2023-10-13)
Supplement: Supplementary file 3 [file 4.1-mixup.tex]

% \subsection{Synthetic dataset with Mixup augmentation}

\subsubsection{Better approximation with proper temperature and interpolation ratio}
\label{sect:better-approximate-mixup}

In Section~\ref{sect:synthetic} we show that on our synthetic dataset with known true distribution, namely mixup augmentation, the model probability can approach the true distribution. In light of our analyses in Section~\ref{sect:approximate-true-distribution}, here we show that with temperature $T$ and interpolation ratio $\lambda$, the model probability can approximate the true label distribution even better.

\smallsection{Temperature}
Here we focus on the effect of temperature on the model at the last checkpoint. We do not experiment on the model at the best checkpoint because we observe that $T=1$ is already near-optimal for best model in this experiment. As shown in Section~\ref{sect:synthetic}, the predictive probability of the model at the last checkpoint (or an overfitted model) cannot approximate the true label distribution well and thus it will produce double descent as significant as the assigned label. However, as shown in Table~\ref{table:augment-distance-temperature}, by properly set the temperature in the softmax function, the predicative probability can still approximate the true label distribution better than the assigned label. Consequently, it will also alleviate the double descent as shown in Figure~\ref{fig:method-augment-temperature}. Here the TV distance is smaller than the best model as we are considering all the examples thus the high accuracy plays a part.

% \chengyu{Best model worse than last model with temperature 10 in terms of TV because we consider all the examples here. Last model has much higher accuracy.}
% One can also find that the TV distance of the predictive distribution is almost as large as the assigned label, indicating a strong miscalibration. This shows quality uncertainty is more important than the accuracy when using predictive distribution as supervision. Interestingly, by tuning the temperature ($T=10$) for overfitted model, one can also better approach the true distribution. And as expected, this carefully selected temperature can help the model alleviate the double descent, which is consistent with our theoretical understanding.

% \begin{wrapfigure}{r}{5.5cm}% [!ht]
%   \centering
%   \includegraphics[width=1.0\linewidth]{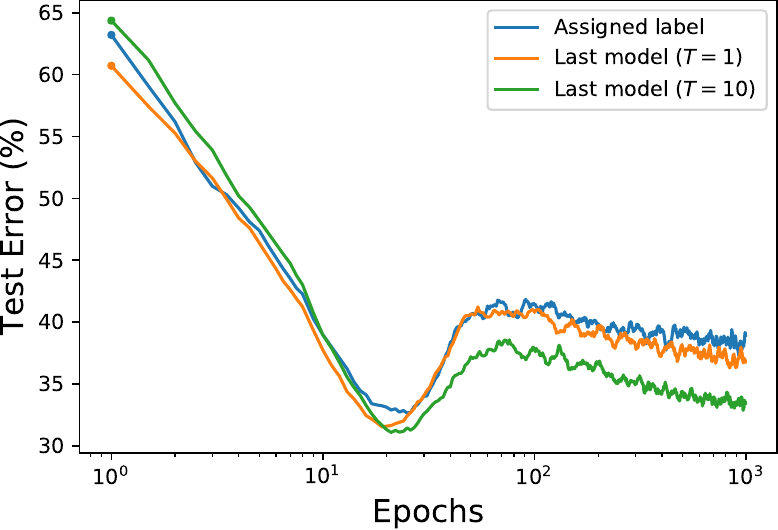}
%   \caption{Test error yielded by standard training on the mixup augmented dataset.  $(\cdot)$ in the legend indicates the distributions employed as the supervision.}%
%   \label{fig:method-augment}
% \end{wrapfigure}

\begin{figure}[!ht]
\begin{floatrow}
\ffigbox{
  \includegraphics[width=1.0\linewidth]{figures/method-augment-temperature.pdf}
  \caption{Test error yielded by standard training on the mixup augmented dataset.  $(\cdot)$ in the legend indicates the distributions employed as the supervision.}%
  \label{fig:method-augment-temperature}
}
\hfill
\capbtabbox{%
  \small
  \begin{tabular}{rlll}
    \toprule
    % & \multicolumn{3}{c}{PGD} & \multicolumn{3}{c}{TRADES}\\
    % \cmidrule(lr){2-4} \cmidrule(lr){5-7}
    % & \specialcell{Robust\\(\%)} & \specialcell{Wall time\\(mins)} & \specialcell{Robust\\(\%)} & \specialcell{Wall time\\(mins)}\\
    Distribution & Acc (\%) & TV & NLL (Val) \\
    \midrule
    Assigned label & 100  & 0.5 & - \\
    \makecell{Last Model \\ ($T=1$)} & 99.84 & 0.4996 & 2.7767 \\
    \makecell{Last Model \\ ($T=10$)} & 99.84 & 0.4315 & 1.2297 \\
    % Last Model ($T$=2) & 99.88 & 0.4388\\
    % Last Model ($T$=10) & 99.84 & 0.4315 & \\
    \bottomrule
    % \tablefootnote{$^*$ indicates the best hyper-parameter searched.}
  \end{tabular}
}{%
  \vspace{8ex}
  \caption{Average TV distance between the true label distribution and various approximate label distributions. The accuracy of the label distribution in terms of the argmax of the true label is also listed for reference.
  % Experiment settings are specified in the text. Unless otherwise noted, we set the temperature to be $1$ in the softmax function, which recovers the original probability of the model.
  }
  \label{table:augment-distance-temperature}
}
\end{floatrow}
\end{figure}

% \begin{wrapfigure}{r}{5.5cm}% [!ht]
%   \centering
%   \includegraphics[width=1.0\linewidth]{figures/method-augment-temperature.pdf}
%   \caption{Test error yielded by standard training on the mixup augmented dataset.  $(\cdot)$ in the legend indicates the distributions employed as the supervision.}%
%   \label{fig:method-augment}
% \end{wrapfigure}

\smallsection{Interpolation ratio}
Now we validate if properly interpolating between model probability and assigned label can better approximate the true label distribution. As shown in Table~\ref{table:augment-distance-ratio}, a proper interpolation ratio can indeed produce a distribution that approaches the true label distribution closer than the model probability only\footnote{We use a surrogate model to calculate NLL loss for the assigned label, see Appendix~\ref{sect:confidence-calibration-assigned} for details.}. Consequently, it can mitigate the double descent more significantly and achieve better performance.

\begin{figure}[!ht]
\begin{floatrow}
\ffigbox{
  \includegraphics[width=1.0\linewidth]{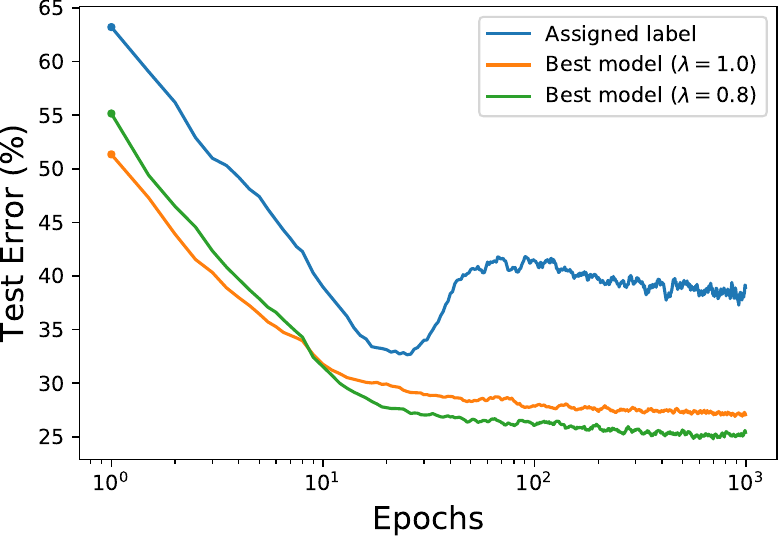}
  \caption{Test error yielded by standard training on the mixup augmented dataset.  $(\cdot)$ in the legend indicates the distributions employed as the supervision.}%
  \label{fig:method-augment-ratio}
}
\hfill
\capbtabbox{%
  \small
  \begin{tabular}{rlll}
    \toprule
    % & \multicolumn{3}{c}{PGD} & \multicolumn{3}{c}{TRADES}\\
    % \cmidrule(lr){2-4} \cmidrule(lr){5-7}
    % & \specialcell{Robust\\(\%)} & \specialcell{Wall time\\(mins)} & \specialcell{Robust\\(\%)} & \specialcell{Wall time\\(mins)}\\
    Distribution & Acc (\%) & TV & NLL (Val) \\
    \midrule
    Assigned label & 100  & 0.5 & - \\
    \makecell{Best Model \\ ($\lambda=1.0$)} & 80.24 & 0.4420 & 0.9504 \\
    \makecell{Best Model \\ ($\lambda=0.8$)} & 91.09 & 0.3772 & 0.8930 \\
    \bottomrule
  \end{tabular}
}{%
  \vspace{8ex}
  \caption{Average TV distance between the true label distribution and various approximate label distributions. The accuracy of the label distribution in terms of the argmax of the true label is also listed for reference.
  }
  \label{table:augment-distance-ratio}
}
\end{floatrow}
\end{figure}
