# Supplementary material for: Label Noise in Adversarial Training: A Novel Perspective to Study Robust Overfitting
Source: arXiv:2110.03135 source file (2023-10-13)
Supplement: Supplementary file 4 [file 4-deprecated.tex]

% \smallsection{Proof of Theorem~\ref{theorem:implicit-label-noise}}
% % This theorem can be easily proven by the \emph{coupling inequality}. 
% % \todo{Not that clear, first show the equivalence between several label distributions by Remark~\ref{remark:common-practice} and the construction of the clean dataset.}


%     % \begin{proof}
%     % This is a result induced by the \emph{coupling inequality}~\cite{Levin2008MarkovCA} (See Appendix~\ref{sect:label-noise-more-proof}).
%     % \end{proof}

% By \emph{coupling inequality} we have
% \begin{equation}
%     P(\tilde{Y}_\delta \ne Y^*_\delta | x_\delta) \ge 
%     \| P(\tilde{Y}_\delta | x_\delta) - P(Y^*_\delta | x_\delta)\|_{TV}   
% \end{equation}
% By definition of the traditional adversarial label~(\ref{remark:common-practice}) we have $P(\tilde{Y}_\delta | x_\delta) = P(Y|x)$. By property of the clean dataset~(\ref{assumption:clean-dataset}) we have $P(Y|x) = P(Y^*|x)$, which together means $P(\tilde{Y}_\delta | x_\delta) = P(Y^*|x)$.
    
% Therefore,        
% \begin{equation}
% P(\tilde{Y}_\delta \ne Y^*_\delta | x_\delta) \ge 
% % \| p(\tilde{Y}_\delta | x_\delta) - p(Y^*_\delta | x_\delta)\|_{TV} = 
% \left\| P(Y^*|x) -  P(Y^*_\delta|x_\delta) \right\|_{\text{TV}}.
% \end{equation}



% % \subsection{Unify implicit label noise and label flipping noise}
% % \label{sect:label-noise-interpret}

% % \note{This is probably not sure. Label flipping noise not necessarily mean the argmax label will be different, but just the probability mass will translate to classes other than the argmax classes. The key difference between implicit and typical label noise is still implicit noise emphasize on instance-dependent, while label noise is typically agnostic of instance, thus it can be applied to the entire dataset as a whole (But it can still be defined instance-wisely.)}
% % \sout{In classification problems, label noise is typically defined in a conditional manner. Specifically, there exists some noise event, such that when it happens, the assigned label is different from the true label.} However, in this paper we have shown that implicit label noise, defined as a mismatch between the true label distribution and the assigned label distribution, is also important and can introduce double descent. In this section we show that it is possible to unify these two types of label noise. We note that there is no need to distinguish a clean example and an adversarial example here.

% % \todo{Show three types of label flipping noise and their connection to implicit label noise.}
% % \todo{Just define this as implicit label noise, otherwise cannot align with the definition in the main paper.}

% \begin{definition}[Generic label noise]
% Given an example $x$, label noise can be defined as the the probability that its assigned label $\hat{y}$ is different from its true label $y$, namely
% \begin{equation}
% \label{eq:generic-label-noise}
%     p \equiv P(\hat{y}\ne y | x)
% \end{equation}
% \end{definition}

% \begin{lemma}
% \label{lemma:generic-label-noise}
% The label noise can be rewritten with the conditional probability, namely
% \begin{equation}
%     \label{eq:generic-label-noise-derive}
%     P(\hat{y}\ne y | x) = 1 - \sum_j P(\hat{y}=j | y = j, x) P(y = j|x).
% \end{equation}
% \end{lemma}
% \begin{proof}
% $$
% \begin{aligned}
%     P(\hat{y}\ne y | x)
%     & = 1 - \sum_j P(\hat{y} = j,  y = j | x) \\
%     & = 1 - \sum_j P(\hat{y}=j | y = j, x) P(y = j|x)\\
% \end{aligned}
% $$
% \end{proof}

% Now we show that the label flipping noise and implicit label noise are special cases of this definition.

% \smallsection{Label flipping noise}
% For simplicity, we consider a type of label flipping noise independent of the true label $y$ and the input $x$, namely 
% $$
% P(\hat{y} \ne j | y=j, x) = \frac{p_e}{c - 1},
% $$
% where $c$ is the number of classes. Lemma~\ref{lemma:generic-label-noise} implies
% $$
% P(\hat{y} \ne y | x) = 1 - (1 - p_e) \sum_j P(y = j | x) = p_e,
% $$
% which degenerates to a constant. Such label noise can be easily interpreted as the fraction of incorrectly labeled examples in the training set. Note here we do not specify the form of true label distribution $P(y = j|x)$.
% % \begin{itemize}
% %     \item Conditional dependence is specified (constant):
% %     $$ P(\hat{y}' | y', x') = p_e$$ 
% %     \item The distribution of the assigned label $P(\hat{y}' | x')$ is arbitrary
% % \end{itemize}

% \smallsection{Implicit label noise}
% In contrast to the above case, implicit label noise specifies the distribution of the assigned label $P(\hat{y} | x)$ and $P(\hat{y} | x) \ne P(y | x)$, leading to a distribution mismatch. The coupling between the assigned label distribution and the true label distribution is unknown, or equivalently, the conditional distribution $P(\hat{y} | y, x)$ can be arbitrary. However, based on the coupling inequality, we can bound the generic label noise as follows
% $$
% P(\hat{y}\ne y | x) \ge \|P(\hat{y}|x) - P(y | x)\|_{\text{TV}},
% $$
% which is same as Theorem~\ref{theorem:implicit-label-noise}.
% % Label noise in adversarial training
% % \begin{itemize}
% %     \item The distribution of the assigned label is specified
% %     $$ P(\hat{y}' | x') = P(y|x),$$
% %     since adversarial training sets $\hat{y}' \equiv \hat{y} \equiv y$. The latter equivalence assumes there is no label noise in the original dataset.
% %     \item Conditional dependence $P(\hat{y}' | y', x')$ is arbitrary
% % \end{itemize}
% % Note that here the conditional dependence is not specified, which means the coupling between $P(\hat{y}'|x')$ and $P(y'|x')$ can be arbitrary.



% \smallsection{Sanity check of Assumption~\ref{eq:label-noise-assumption}}
% Here we check if Assumption~\ref{eq:label-noise-assumption} is reasonable by studying a Gaussian mixture model (GMM).

% % \begin{example}[Gaussian Mixture Model]
% The conditional distribution in a Gaussian mixture model can be formulated as
%   $$
%   P(Y=j|x) \equiv f^*(x)_j = \frac{\psi_j \mathcal{N}_x(\mu_j, \sigma_j)}{\sum_l \psi_l \mathcal{N}_x(\mu_l, \sigma_l)} \equiv \frac{\psi_j g_j(x)}{\sum_l \psi_l g_l(x)},
%   $$

%   where
%   $$
%   g_l(x) = \frac{1}{\sqrt{\text{det}(2\pi\sigma_l)}}\exp\left[-\frac{1}{2}(x - \mu_l)^T\sigma_l^{-1}(x-\mu_l)\right].
%   $$

%   The gradient can be derived as
%   $$
%   \begin{aligned}
%   \nabla_x f^*(x)_j 
%   & = \frac{\psi_j\nabla g_j(x)}{\sum_l \psi_l g_l(x)} - \psi_jg_j(x)\frac{\sum_l \psi_l\nabla g_l(x)}{\left[\sum_l \psi_lg_l(x)\right]^2}\\
%   & = \frac{- \psi_j g_j(x)\sigma_j^{-1}(x - \mu_j)}{\sum_l \psi_l g_l(x)} +  \psi_jg_j(x)\frac{\sum_l \psi_l g_l(x)\sigma_l^{-1}(x - \mu_l)}{\left[\sum_l \psi_l g_l(x)\right]^2}\\
%   & = \frac{\psi_j g_j(x)}{\sum_l \psi_l g_l(x)} \left[-\sigma_j^{-1} (x - \mu_j)  +  \frac{\sum_l \sigma_l^{-1}(x - \mu_l) \psi_l g_l(x)}{\sum_l \psi_l g_l(x)}\right]\\
%   & = f^*(x)_j \left[-\sigma_j^{-1} (x - \mu_j) + \sum_l f^*(x)_l \sigma_l^{-1}(x - \mu_l)\right]\\
%   \end{aligned}
%   $$

% When $x - \mu_j \to 0$, $f^*(x)_j \to 1$ and $f^*(x)_l \to 0$, for $l\ne j$,
% $$
% \nabla_x f^*(x)_j \approx f^*(x)_j(f^*(x)_j - 1)\sigma_j^{-1} (x - \mu_j)
% $$
% Therefore
% $$
% \|\nabla_x f^*(x)_j \| \propto 1 - f^*(x)_j
% $$

% % \end{example}

% % *Reference*:
% % * Matrix cookbook
% % * https://web.stanford.edu/~lmackey/stats306b/doc/stats306b-spring14-lecture2_scribed.pdf


% \smallsection{Proof of Proposition~\ref{proposition:label-noise}}

% \begin{proof}
% $$
% \begin{aligned}
%     P(Y\ne Y^* | x)
%     & = 1 - \sum_j P(Y = j,  Y^* = j | x) \\
%     & = 1 - \sum_j P(Y=j | Y^* = j, x) P(Y^* = j|x)\\
%     & = 1 - \sum_j (1 - P(Y\ne j | Y^* = j, x)) P(Y^* = j|x)\\
% \end{aligned}
% $$
% \end{proof}
